# Supplementary material for: Scalable and Cost-effective Data Flow Analysis for Distributed Software: Algorithms and Applications
Source: arXiv:2303.03659 source file (2023-03-07)
Supplement: Supplementary file 1 [file appendixa.tex]

\chapter{Appendix A - Some Text}

Some appendix text.
